# Supplementary material for: PQ-NET: A Generative Part Seq2Seq Network for 3D Shapes
Source: arXiv:1911.10949 source file (2020-04-24)
Supplement: Supplementary file 1 [file completion.tex]

% -*- compile-command: "texify --pdf --quiet decop_cvpr18.tex" -*-
% !TEX root = decop_cvpr18.tex
% (shell-command "start decop_cvpr18.pdf")

\section{Partial Shape Completion}
\label{sec:completion}
See results in Figure \ref{fig:complement-more}.

\begin{figure}[htbp]
\begin{center}
\includegraphics[width=\linewidth, height=0.9\linewidth]{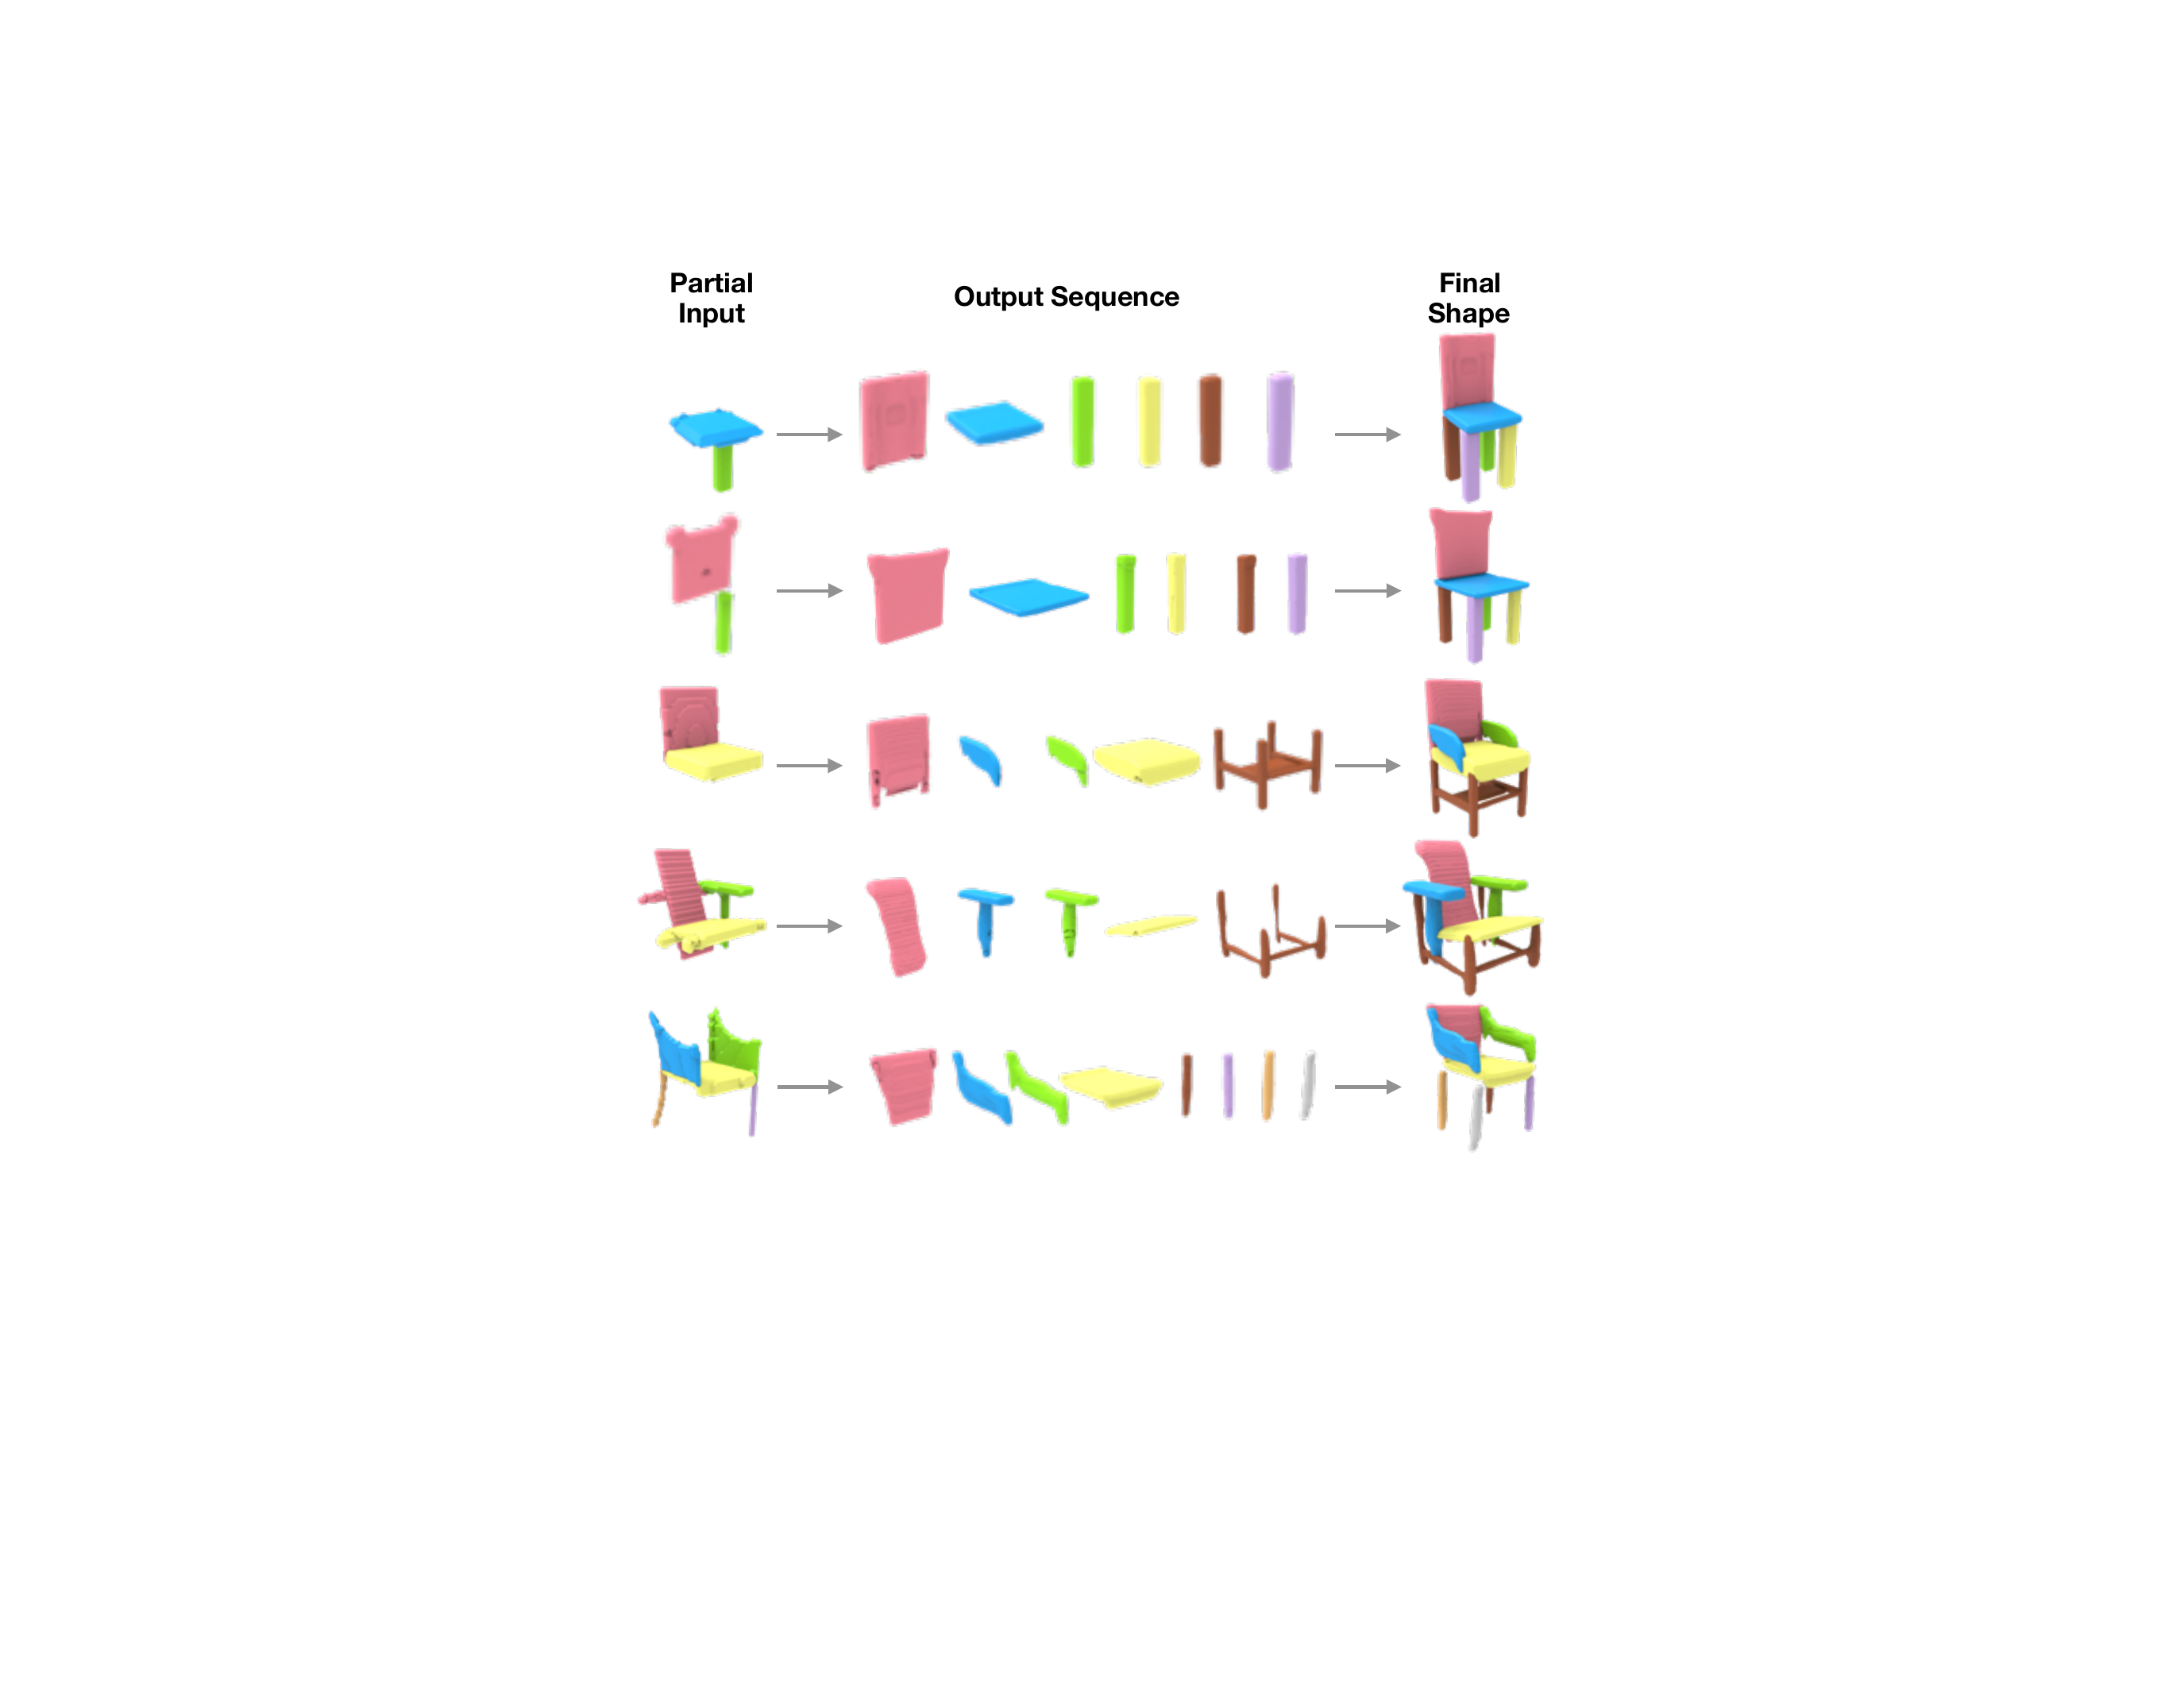}
\end{center}
   \caption{Visual results of partial shape completion.}
\label{fig:complement-more}
\end{figure}
